# Supplementary material for: Orientation Keypoints for 6D Human Pose Estimation
Source: arXiv:2009.04930 source file (2021-12-16)
Supplement: Supplementary file 1 [file supplementary.tex]

\appendices

% \begin{figure*}[ht!]
% \begin{center}
% \includegraphics[width=0.9\textwidth]{latex/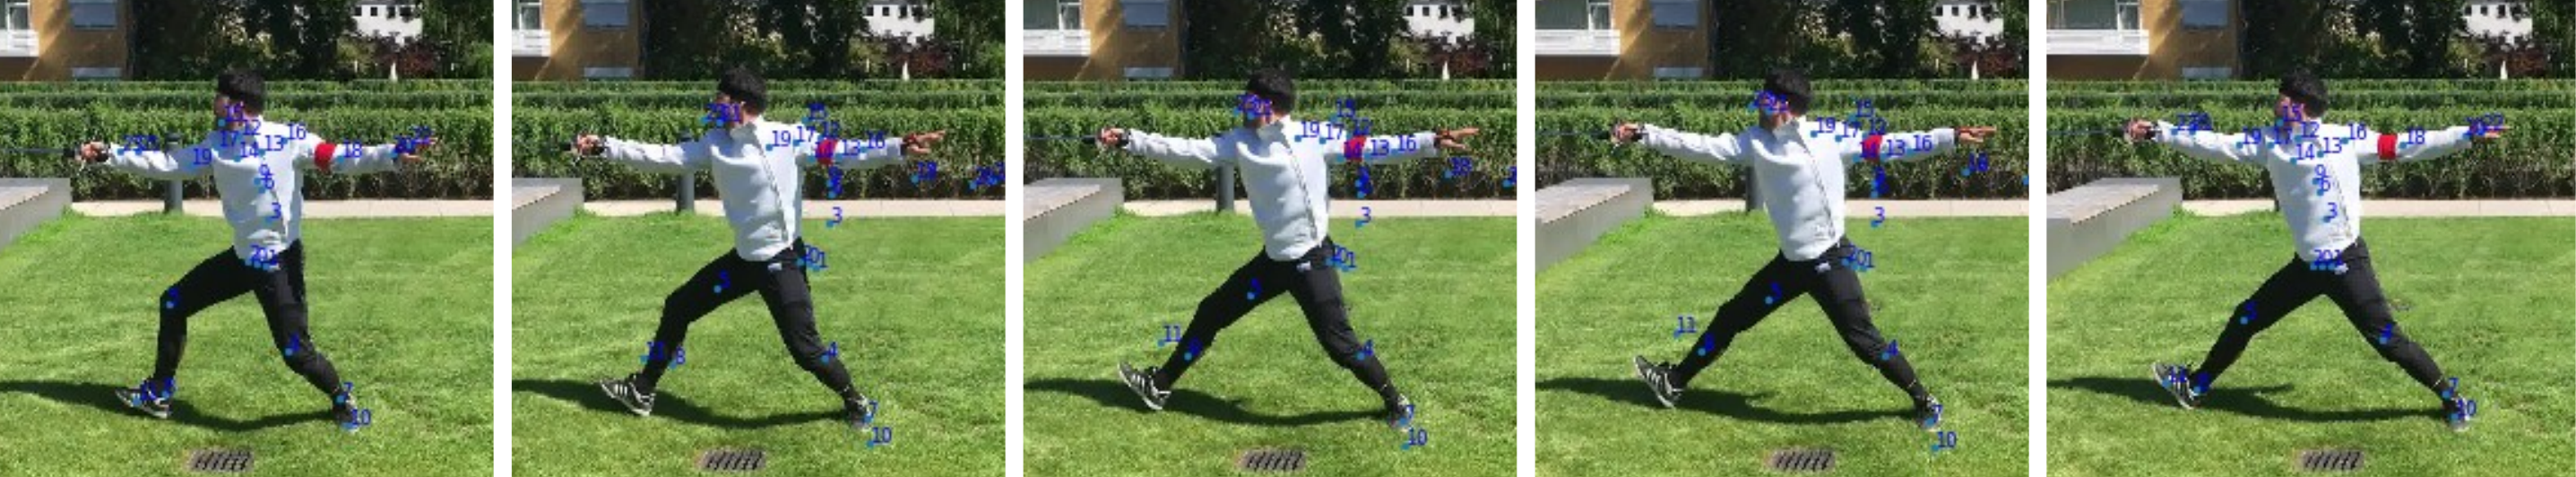}
% \caption{A sequence from the test 3DPW test set with the provided "ground truth" \textit{jointPositions} field projected based on the intrinsics.  The ground truth annotations keypoints detach from the image during a fast motion (middle frames) before snapping back to alignment.  The provided 2D "coco-style" annotations also show a similar jump.}
% \label{Fig: dpw_error}
% \end{center}
% \end{figure*}

% \section{Visualizations of video clips}
% We visualize the skeletal animation of three 20-second video clips taken at 25 fps of one of the Human 3.6m validation subjects in the included supplementary video file.  We show the animation from 360 degree perspective.  We use the rotation predictions from the Crosshairs detector (no refiner) mapped to the average training skeleton.  Each frame is calculated independently, with no intertemporal smoothing applied, yet the animations and rotations are quite smooth.\newline

% \section{Visualizations in the Wild}
% We show more visualization from the MPII test set in Figure \ref{Fig: wild}, all of which are very different subjects, actions and settings from the Human 3.6m training set.  Occlusion is often the biggest issue, as are unfamiliar kneeling poses and generally underestimating the degree of stretch or extension.\newline
